# Supplementary material for: Stable-SCore: A Stable Registration-based Framework for 3D Shape Correspondence
Source: arXiv:2503.21766 source file (2025-03-27)
Supplement: Supplementary file 1 [file supp.tex]

\section{Overview}
This supplementary material includes the following: 
\begin{itemize}
    \item A supplementary video.
    \item More results generated by our method.
\end{itemize}
% (1) A supplementary video. (2) More results generated by our method. 

\section{Video}
Thanks to the robust performance of our approach, our method effectively produces accurate 3D correspondences between characters, enabling various applications such as re-topology, shape interpolation, and rigging \& motion transfer. %We attach a video that showcase these applications. This video includes the registration process (00:31 to 00:49). It also includes several downstream applications empowered by our methods such as Re-topology (00:49 to 01:13), Shape Interpolation (01:41 - 01:34) and Rig\&Motion Transfer (01:34 - 01:52).

% \paragraph{Registration Process} We show the intermediate results during the 5,000 iterations of the registration process. The source mesh smoothly deforms towards the target mesh.

% \paragraph{Re-topology} We show that our method is capable of re-topology. Specifically, we choose meshes from the 3DBiCar \cite{luo2023rabit} dataset, which has a nice topology designed by professional artists. We can transfer such topology to the target mesh using our Stable-Score method. 

% \paragraph{Shape Interpolation} We first register a mesh using Stable-Score from 3DBiCar\cite{luo2023rabit} to any target meshes from our Character in-the-wild (CharW) benchmark dataset. Then, we randomly select two meshes from CharW and conduct shape interpolation between their registered results.

% \paragraph{Rig~\&~Motion Transfer} Using Stable-Score, We are able to transfer the rigging from the SMPL\cite{SMPL:2015} or 3DBiCar\cite{luo2023rabit} to any target meshes in CharW. Two target mesh examples in the video are text-to-3D generated meshes. More specifically, we firstly finds 3d correspondence between the two meshes. Then, compute the joints location by the weighted sum of the related vertex (provided by SMPL and 3DBiCar as joint regressor matrix). The skinning weights can be directed trasfer by the correspondence.
% Finally, we can directly use motion capture sequences to drive these target meshes. The smooth animation indicates the superior performance of our Stable-Score.

We include a video demonstrating these applications. The video covers: \begin{itemize} \item \textbf{Registration process} (00:31–00:49): Intermediate results during the 5,000 iterations of registration are shown, illustrating how the source mesh smoothly deforms towards the target mesh. \item \textbf{Re-topology} (00:49–01:13): Our method successfully transfers the topology of meshes from the 3DBiCar dataset \cite{luo2023rabit}, which features professional-grade topology, to target meshes using our Stable-Score framework. \item \textbf{Shape interpolation} (01:13–01:34): We perform shape interpolation between two randomly selected meshes from the Character in-the-Wild (CharW) benchmark dataset after registering them using Stable-Score. \item \textbf{Rigging \& Motion Transfer} (01:34–01:52): Stable-Score enables the transfer of rigging from SMPL \cite{SMPL:2015} or 3DBiCar \cite{luo2023rabit} models to target meshes from the CharW dataset, including text-to-3D-generated meshes. Using our method, we establish 3D correspondences between meshes, compute joint locations via a weighted sum of related vertices (derived from SMPL or 3DBiCar joint regressors), and directly transfer skinning weights. This allows seamless application of motion capture sequences to drive target meshes, with smooth animations showcasing the superior performance of Stable-Score. \end{itemize}

\input{figures_tex/supp_d4th}

\input{figures_tex/supp_charw1}
\input{figures_tex/supp_charw2}
\input{figures_tex/supp_charw3}

\section{More results}
More results on the DT4D dataset and CharW dataset are shown in Figure~\ref{fig:DT4D}, \ref{fig:charw1}, \ref{fig:charw2} and \ref{fig:charw3}. It can be observed that our Stable-Score achieves precise registration while simultaneously preserving the source topology, thereby demonstrating significant potential for re-topology applications.
